# Supplementary material for: Bridging Physics-based and Data-driven modeling for Learning Dynamical Systems
Source: arXiv:2011.10616 source file (2021-04-29)
Supplement: Supplementary file 1 [file Supplement.tex]

\section{Additional Experiments Details} \label{experiments_details}
We use L2 loss for training and all hyperparamters, including number of layers, hidden dimension and learning rate, are tuned exhaustively on the validation set.

\paragraph{\textit{Sine}} We generate 2000 samples of length 60 from $\sin(wt + b)$. We set step size as 0.2, frequency $w \sim U(0.5, 1.5)$ and phase $b \sim U(0, 5)$. We shuffle and split these samples into 1200 training samples, 400 validation samples and 400 interpolation test samples. 

\paragraph{\textit{SEIR}}  We generate 6000 synthetic \textit{SEIR} time series of length 60 based on Equ \ref{equ-seir} with \textit{scipy.integrate.odeint} with various parameters $\beta, \sigma, \gamma$ and initial value $I_0$. First, we split all samples into a training set, a validation set, an interpolation test set and extrapolation test set based on the range of $\beta$. The training/validation/interpolation-test sets have the same range of $\beta \sim U(0.45, 0.9)$.  The extrapolation-test set contains time series with $\beta \sim U(0.3, 0.45)$. The DL models are trained to make 40-step ahead predictions given the first 20 steps as input. We remove the trend of the trajectories of four variables by differencing.  Then we investigate if the DL models can extrapolate to different initial $I$, so we also try training the models on times series with $I \sim U(30, 100)$, and test them on an $I_0$-interpolation test set where $I \sim U(30, 100)$ and an $I_0$-extrapolation test set where $I \sim U(1, 30)$.

\begin{figure}[H]
\begin{floatrow}
\ffigbox[0.49\textwidth]
{%
	\includegraphics[width=0.24\textwidth]{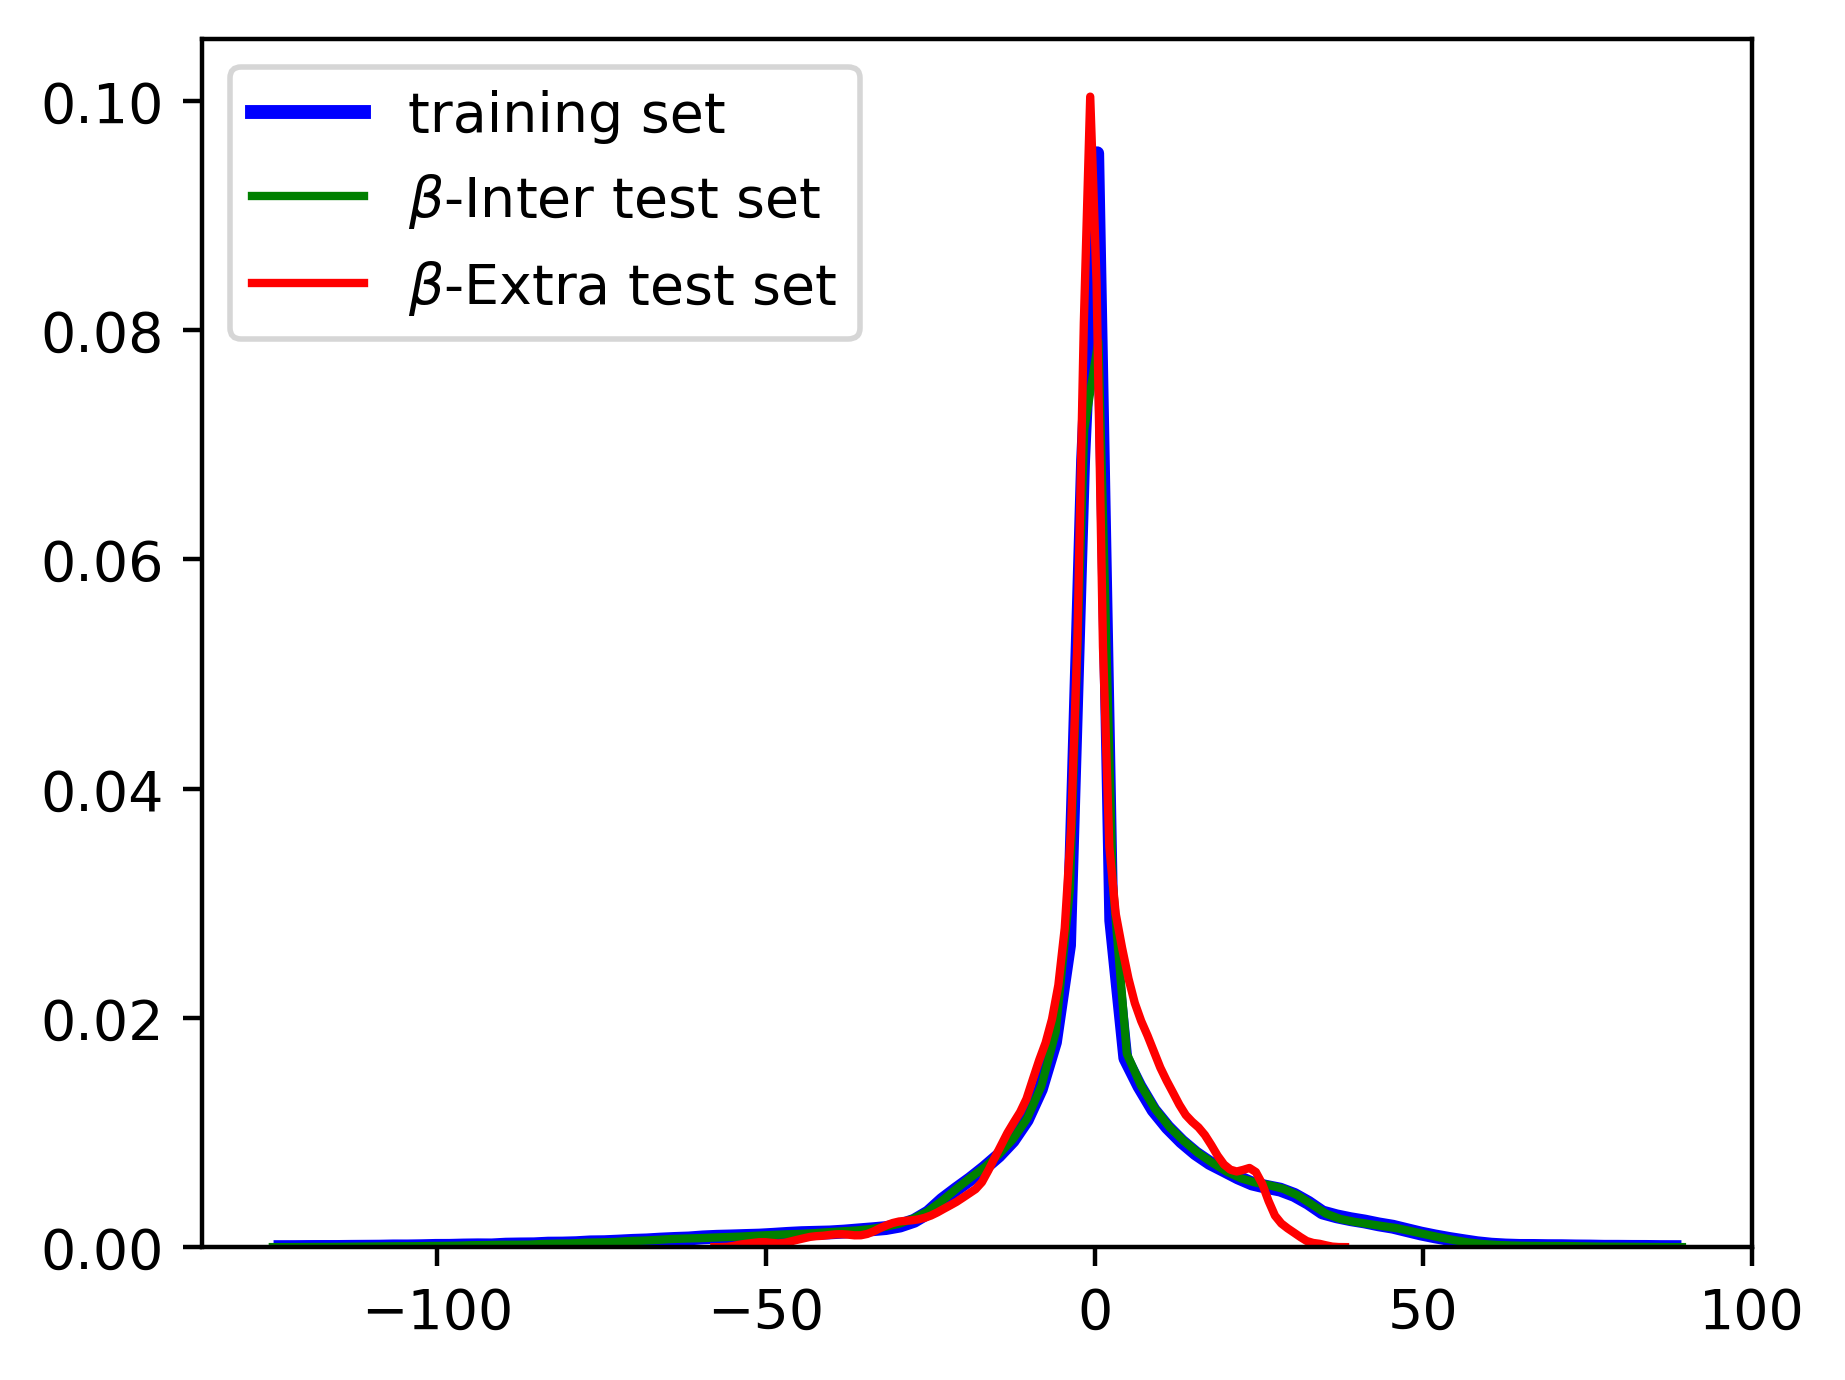}
	\includegraphics[width=0.24\textwidth]{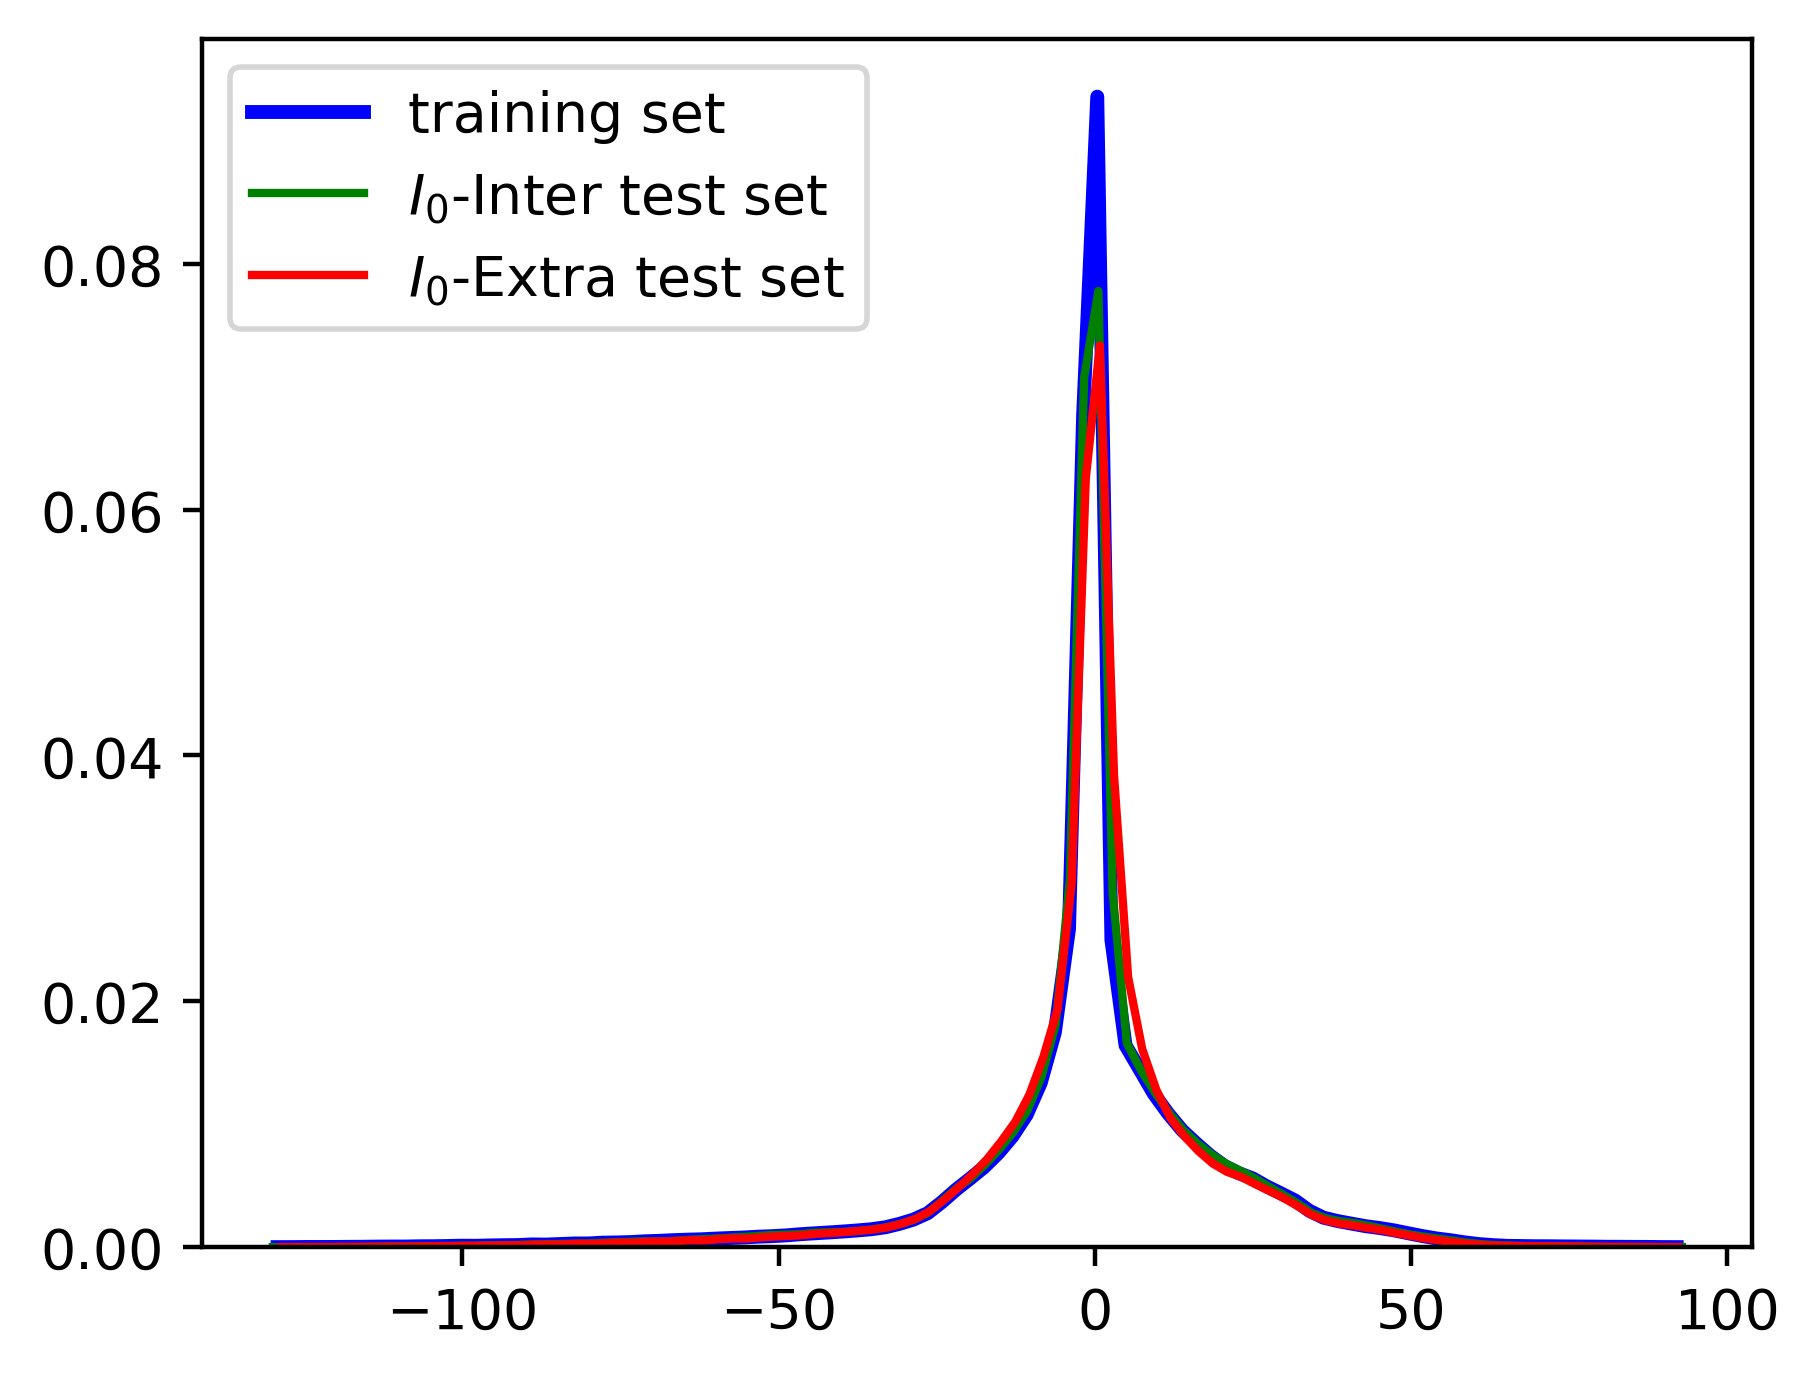}
}{
\caption{The data distribution of the training, $\beta(I_0)$-interpolation and $\beta(I_0)$-extrapolation test sets}\label{fig_dist_seir}
}
\ffigbox[0.49\textwidth]
{%
	\includegraphics[width=0.236\textwidth]{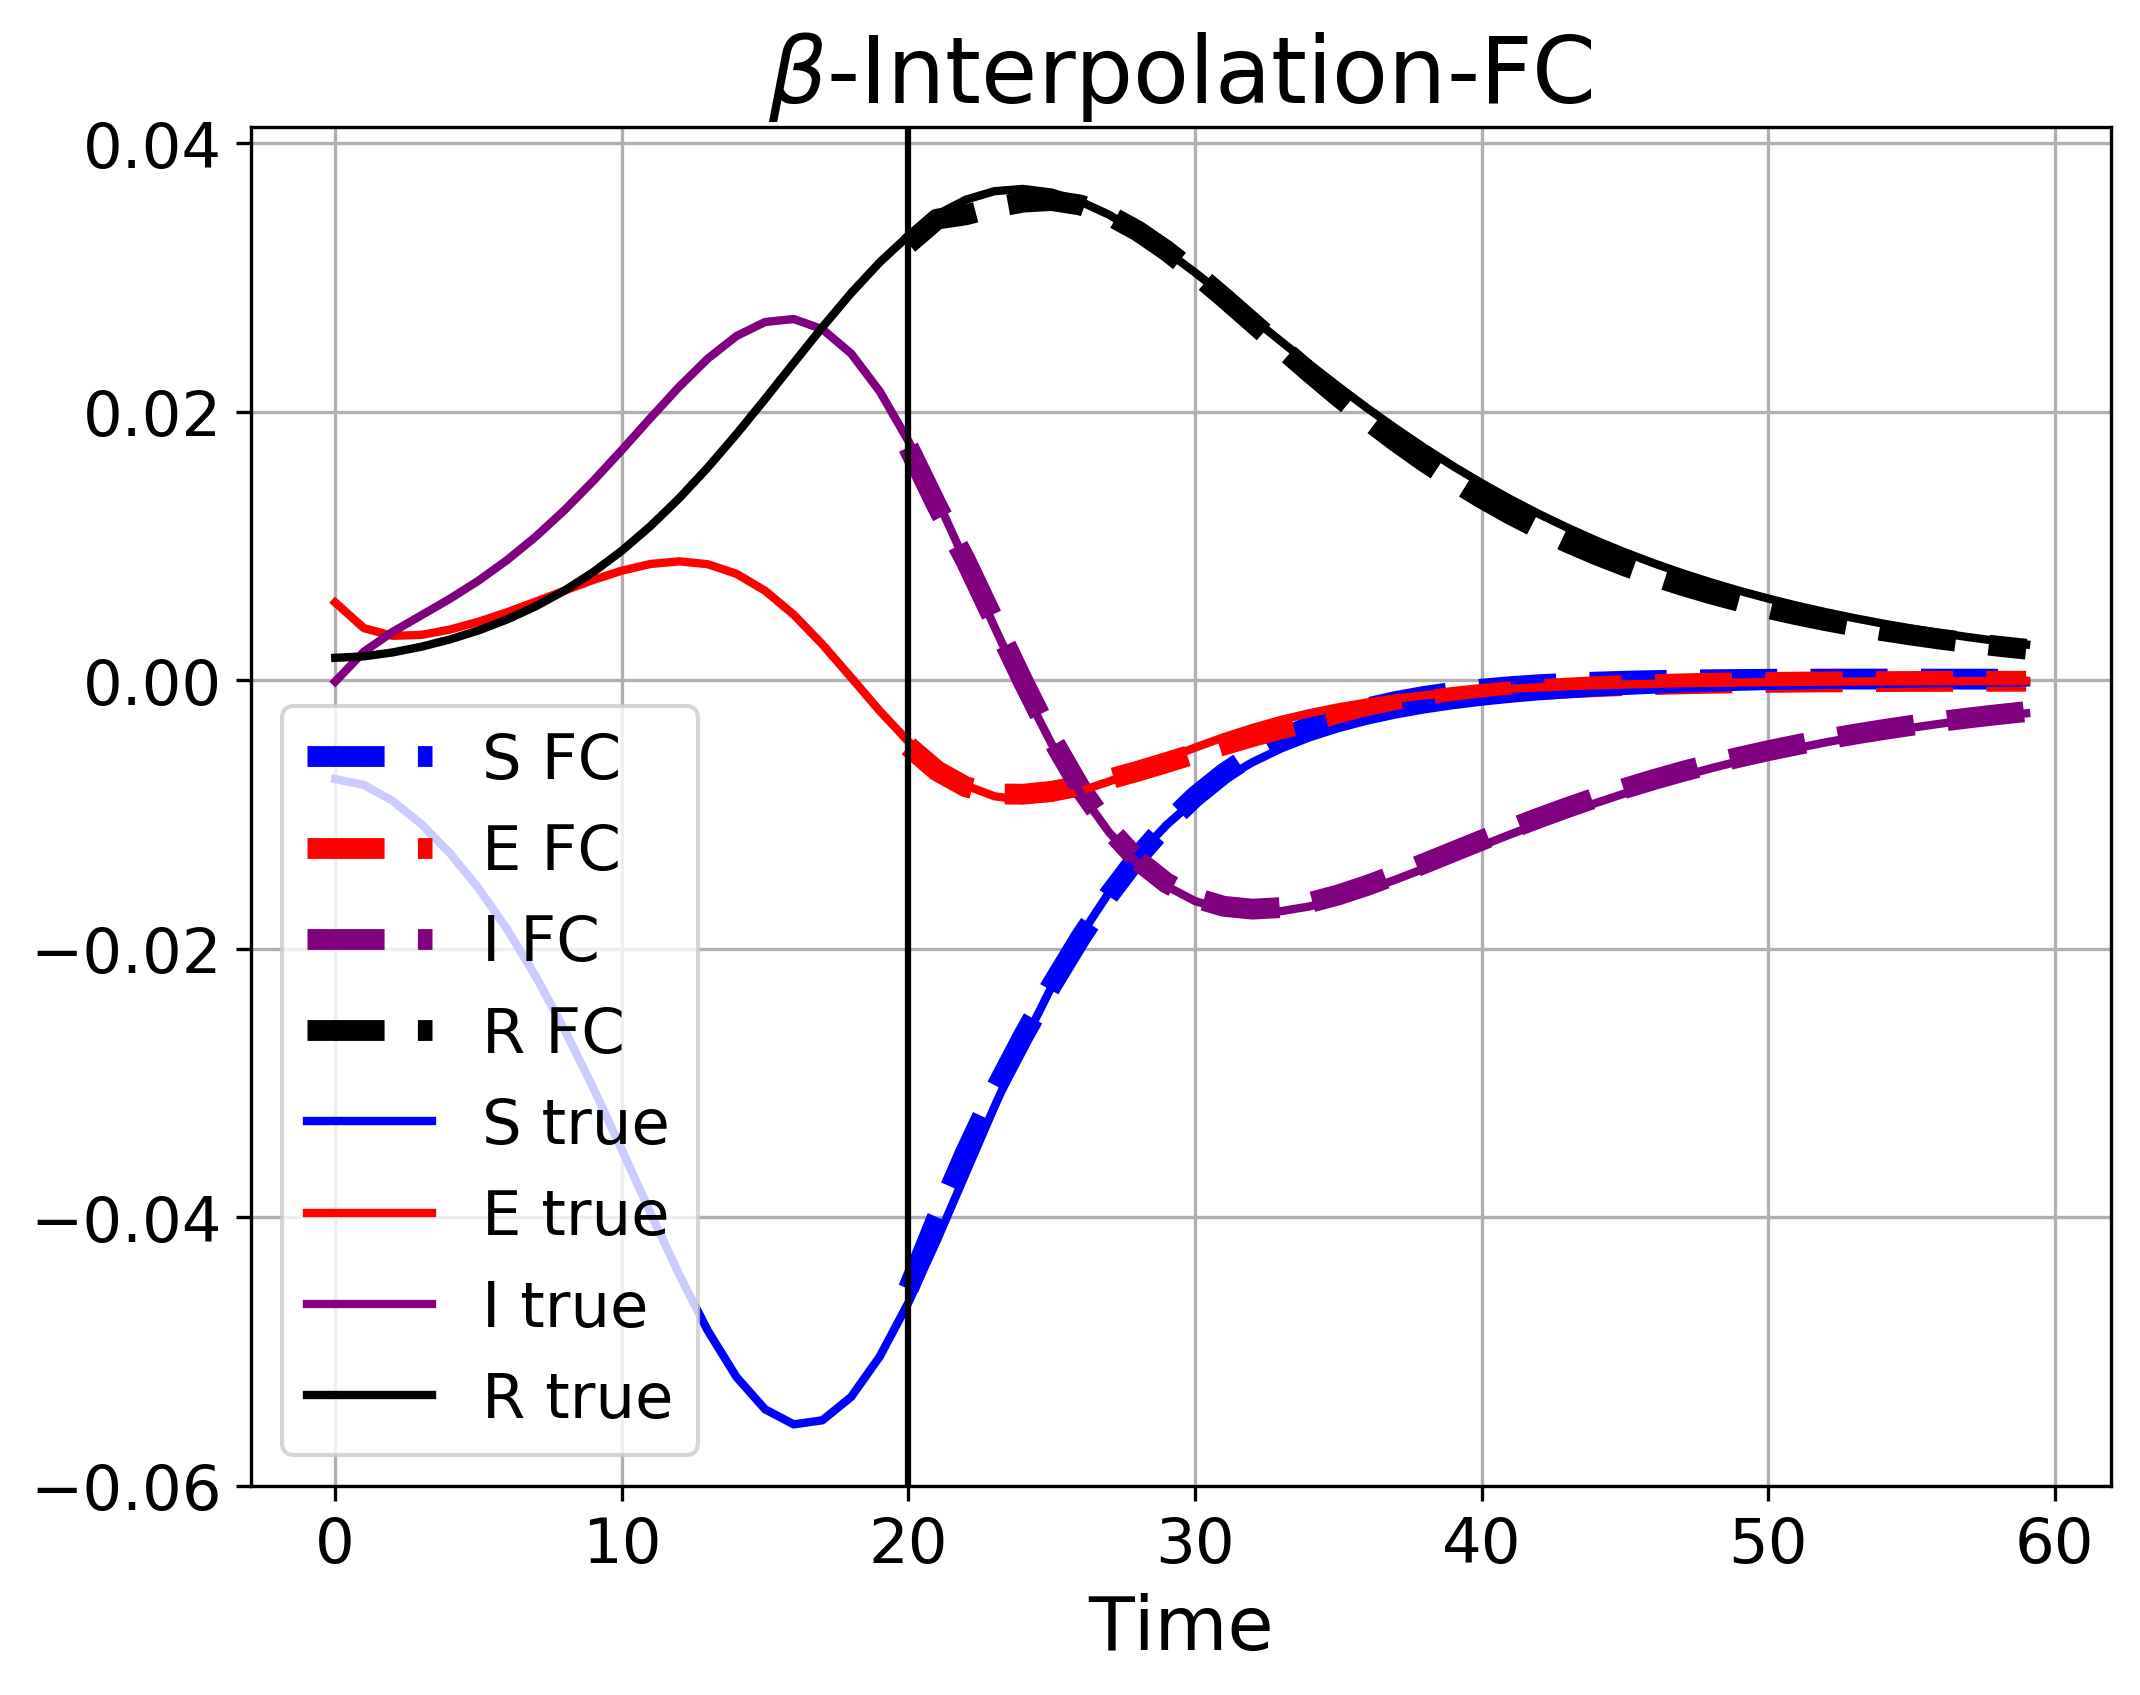}
	\includegraphics[width=0.236\textwidth]{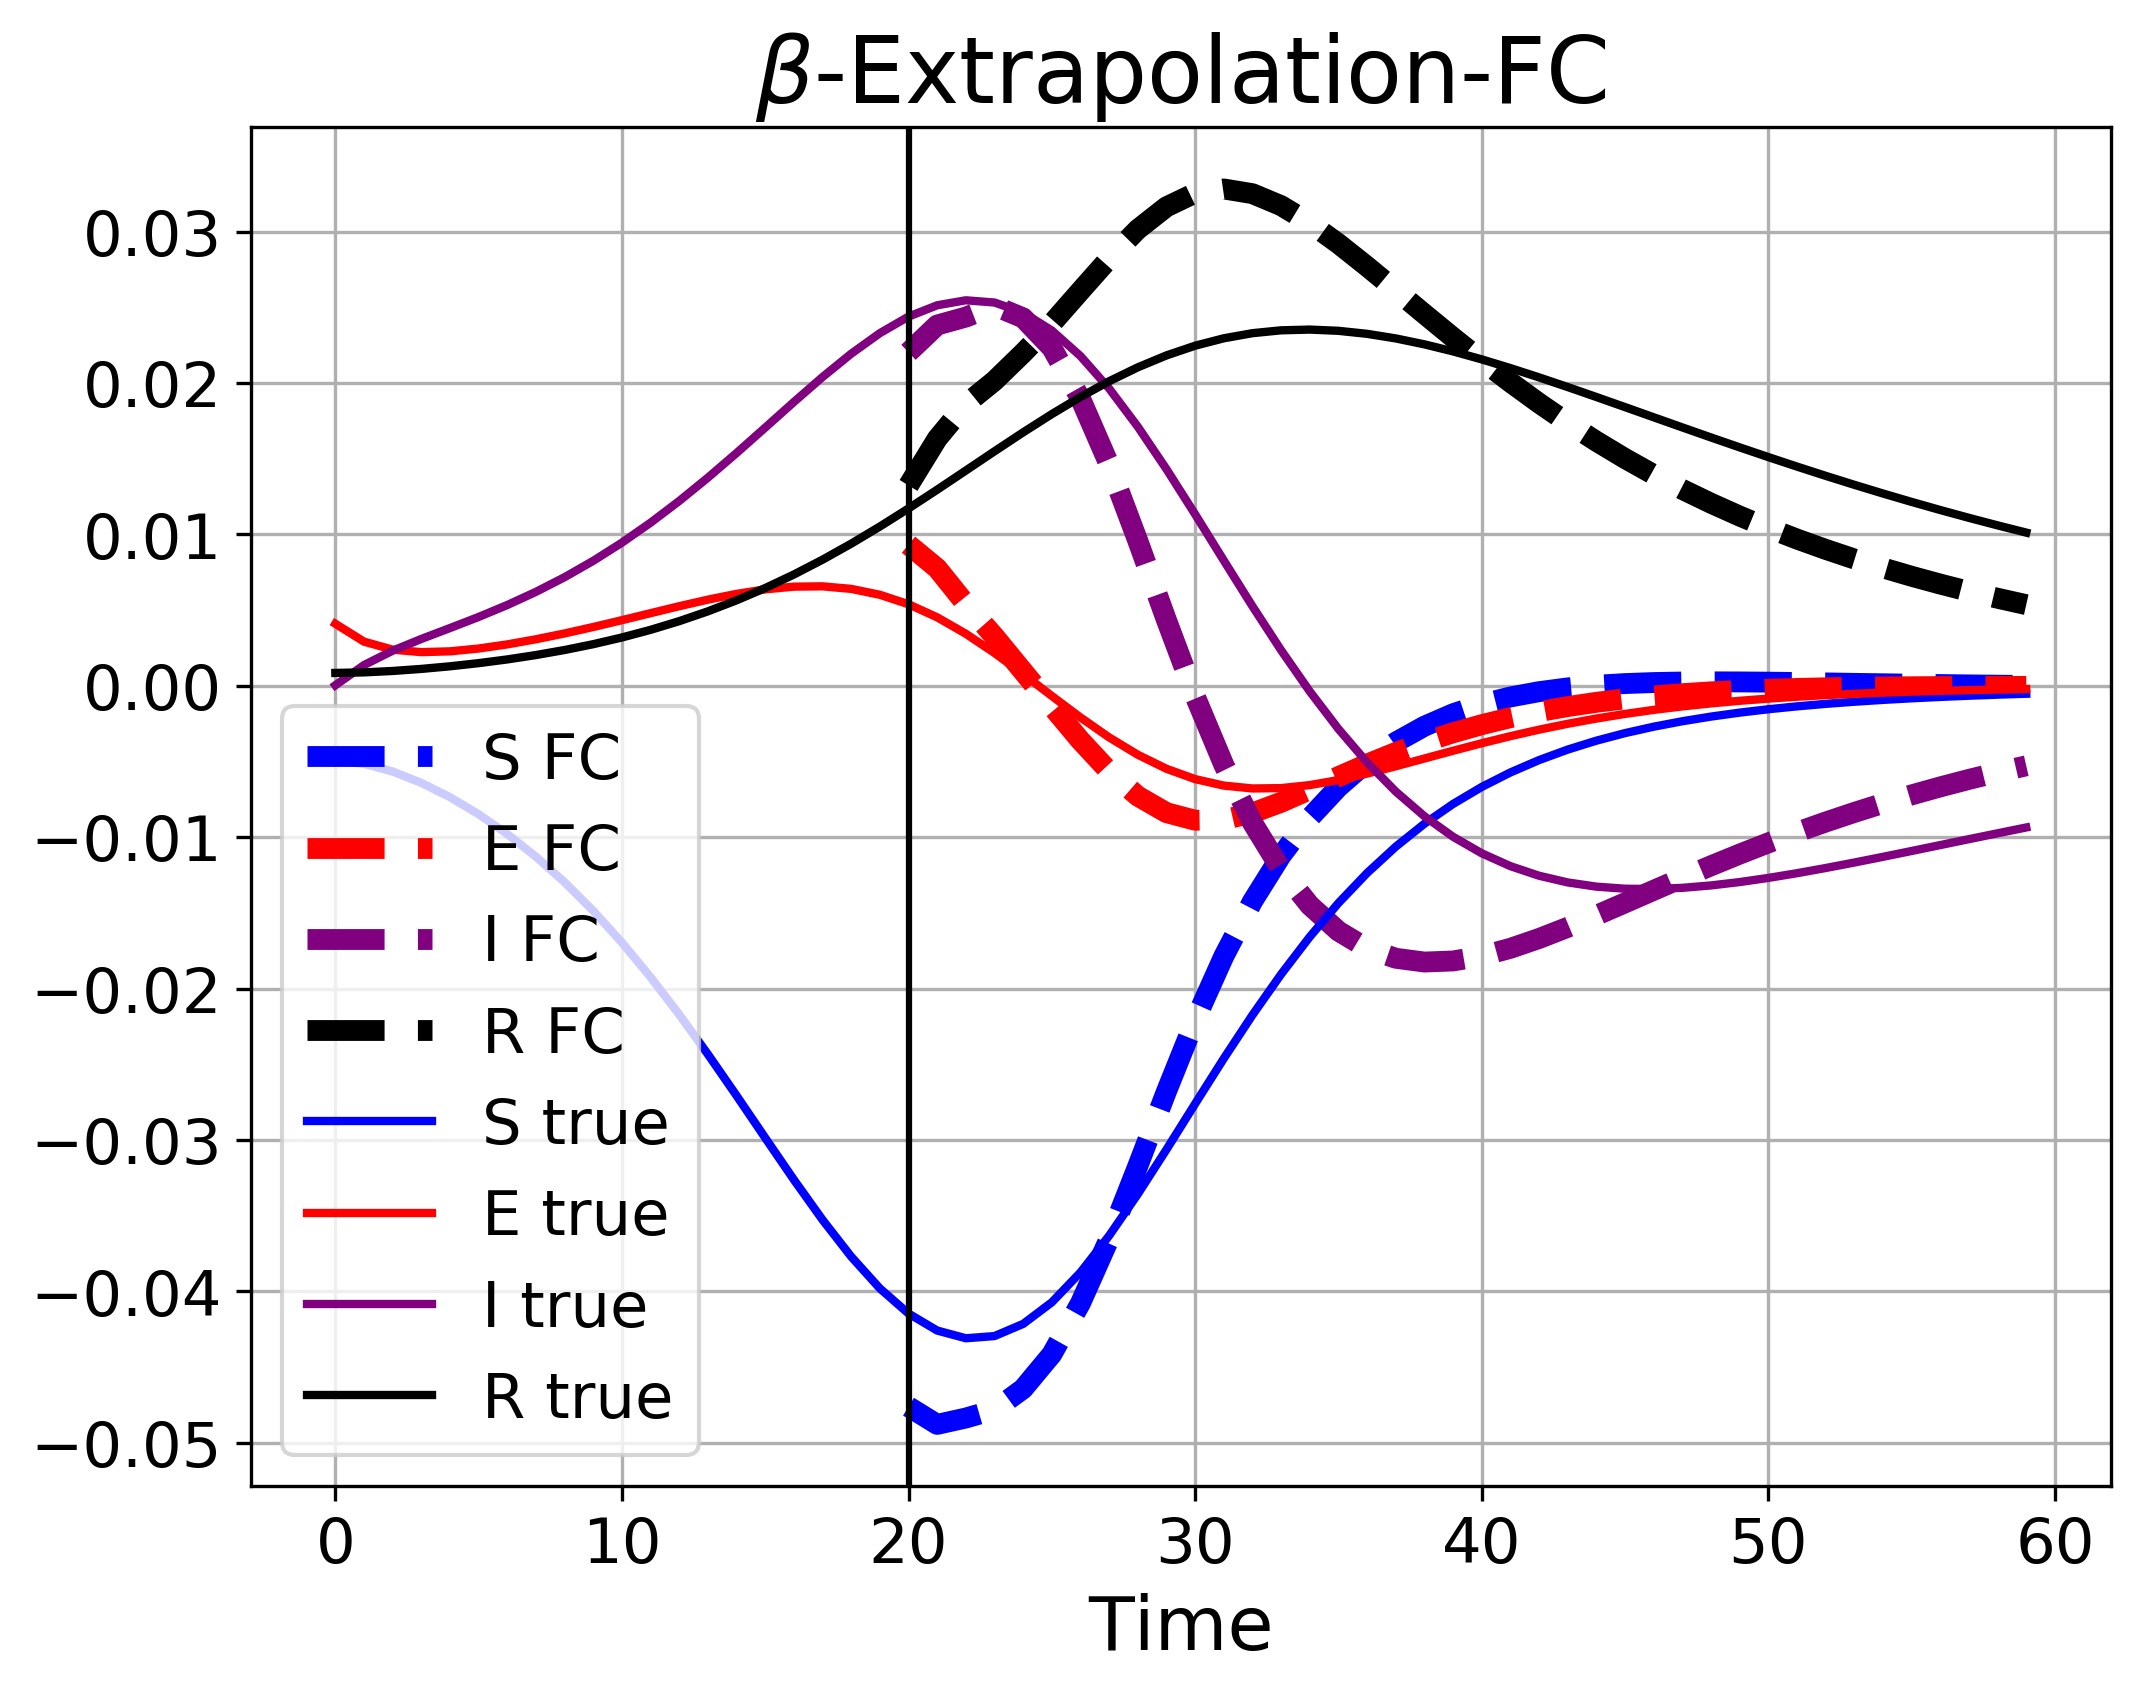}
}{
\caption{\texttt{FC} predictions on a $\beta$-interpolation (left) and a $\beta$-extrapolation (right) test samples of \textit{SEIR} dynamics, the vertical black line in the plots separates the input and forecasting period.}\label{fig_vis_seir}
}
\end{floatrow}
\end{figure}

\paragraph{\textit{LV}} We generate 6000 synthetic 4D \textit{LV} time series of length 20. We normalize each sample so that all values are within the range of 0 and 1. The training/validation/interpolation-test sets have the same range of $\bm{k} \sim U(0, 250)^4$, the and extrapolation-test set contains time series with $\bm{k} \sim U(250, 300)^4$. We also investigate if the DL models can extrapolate to different initial values $\bm{p_0}$. We also train the models on samples with $\bm{p_0} \sim U(30, 200)^4$ and test them on $\bm{p_0} \sim U(0, 30)^4$ with same experimental setup.  

\paragraph{\textit{FNH}} We generate 6000 synthetic \textit{FNH} time series of length 50. Same as before, we test if the DL models can generalize to different range of parameters and initial values. The models are trained to make 25-step ahead predictions given the first 25 steps as input. $c$-interpolation test set contains sample with $c \sim U(1.5, 5)$ and $c$-extrapolation test set contains samples with $c \sim U(0.5, 1.5)$. $x_0$-interpolation test set contains sample with $x_0 \sim U(2, 10)$ and $x_0$-extrapolation test set contains sample with $x_0 \sim U(0, 2)$. 

\section{AutoODE: additional details}\label{covid}

\begin{figure}[htb!]
	\centering
	\includegraphics[width=0.7\textwidth]{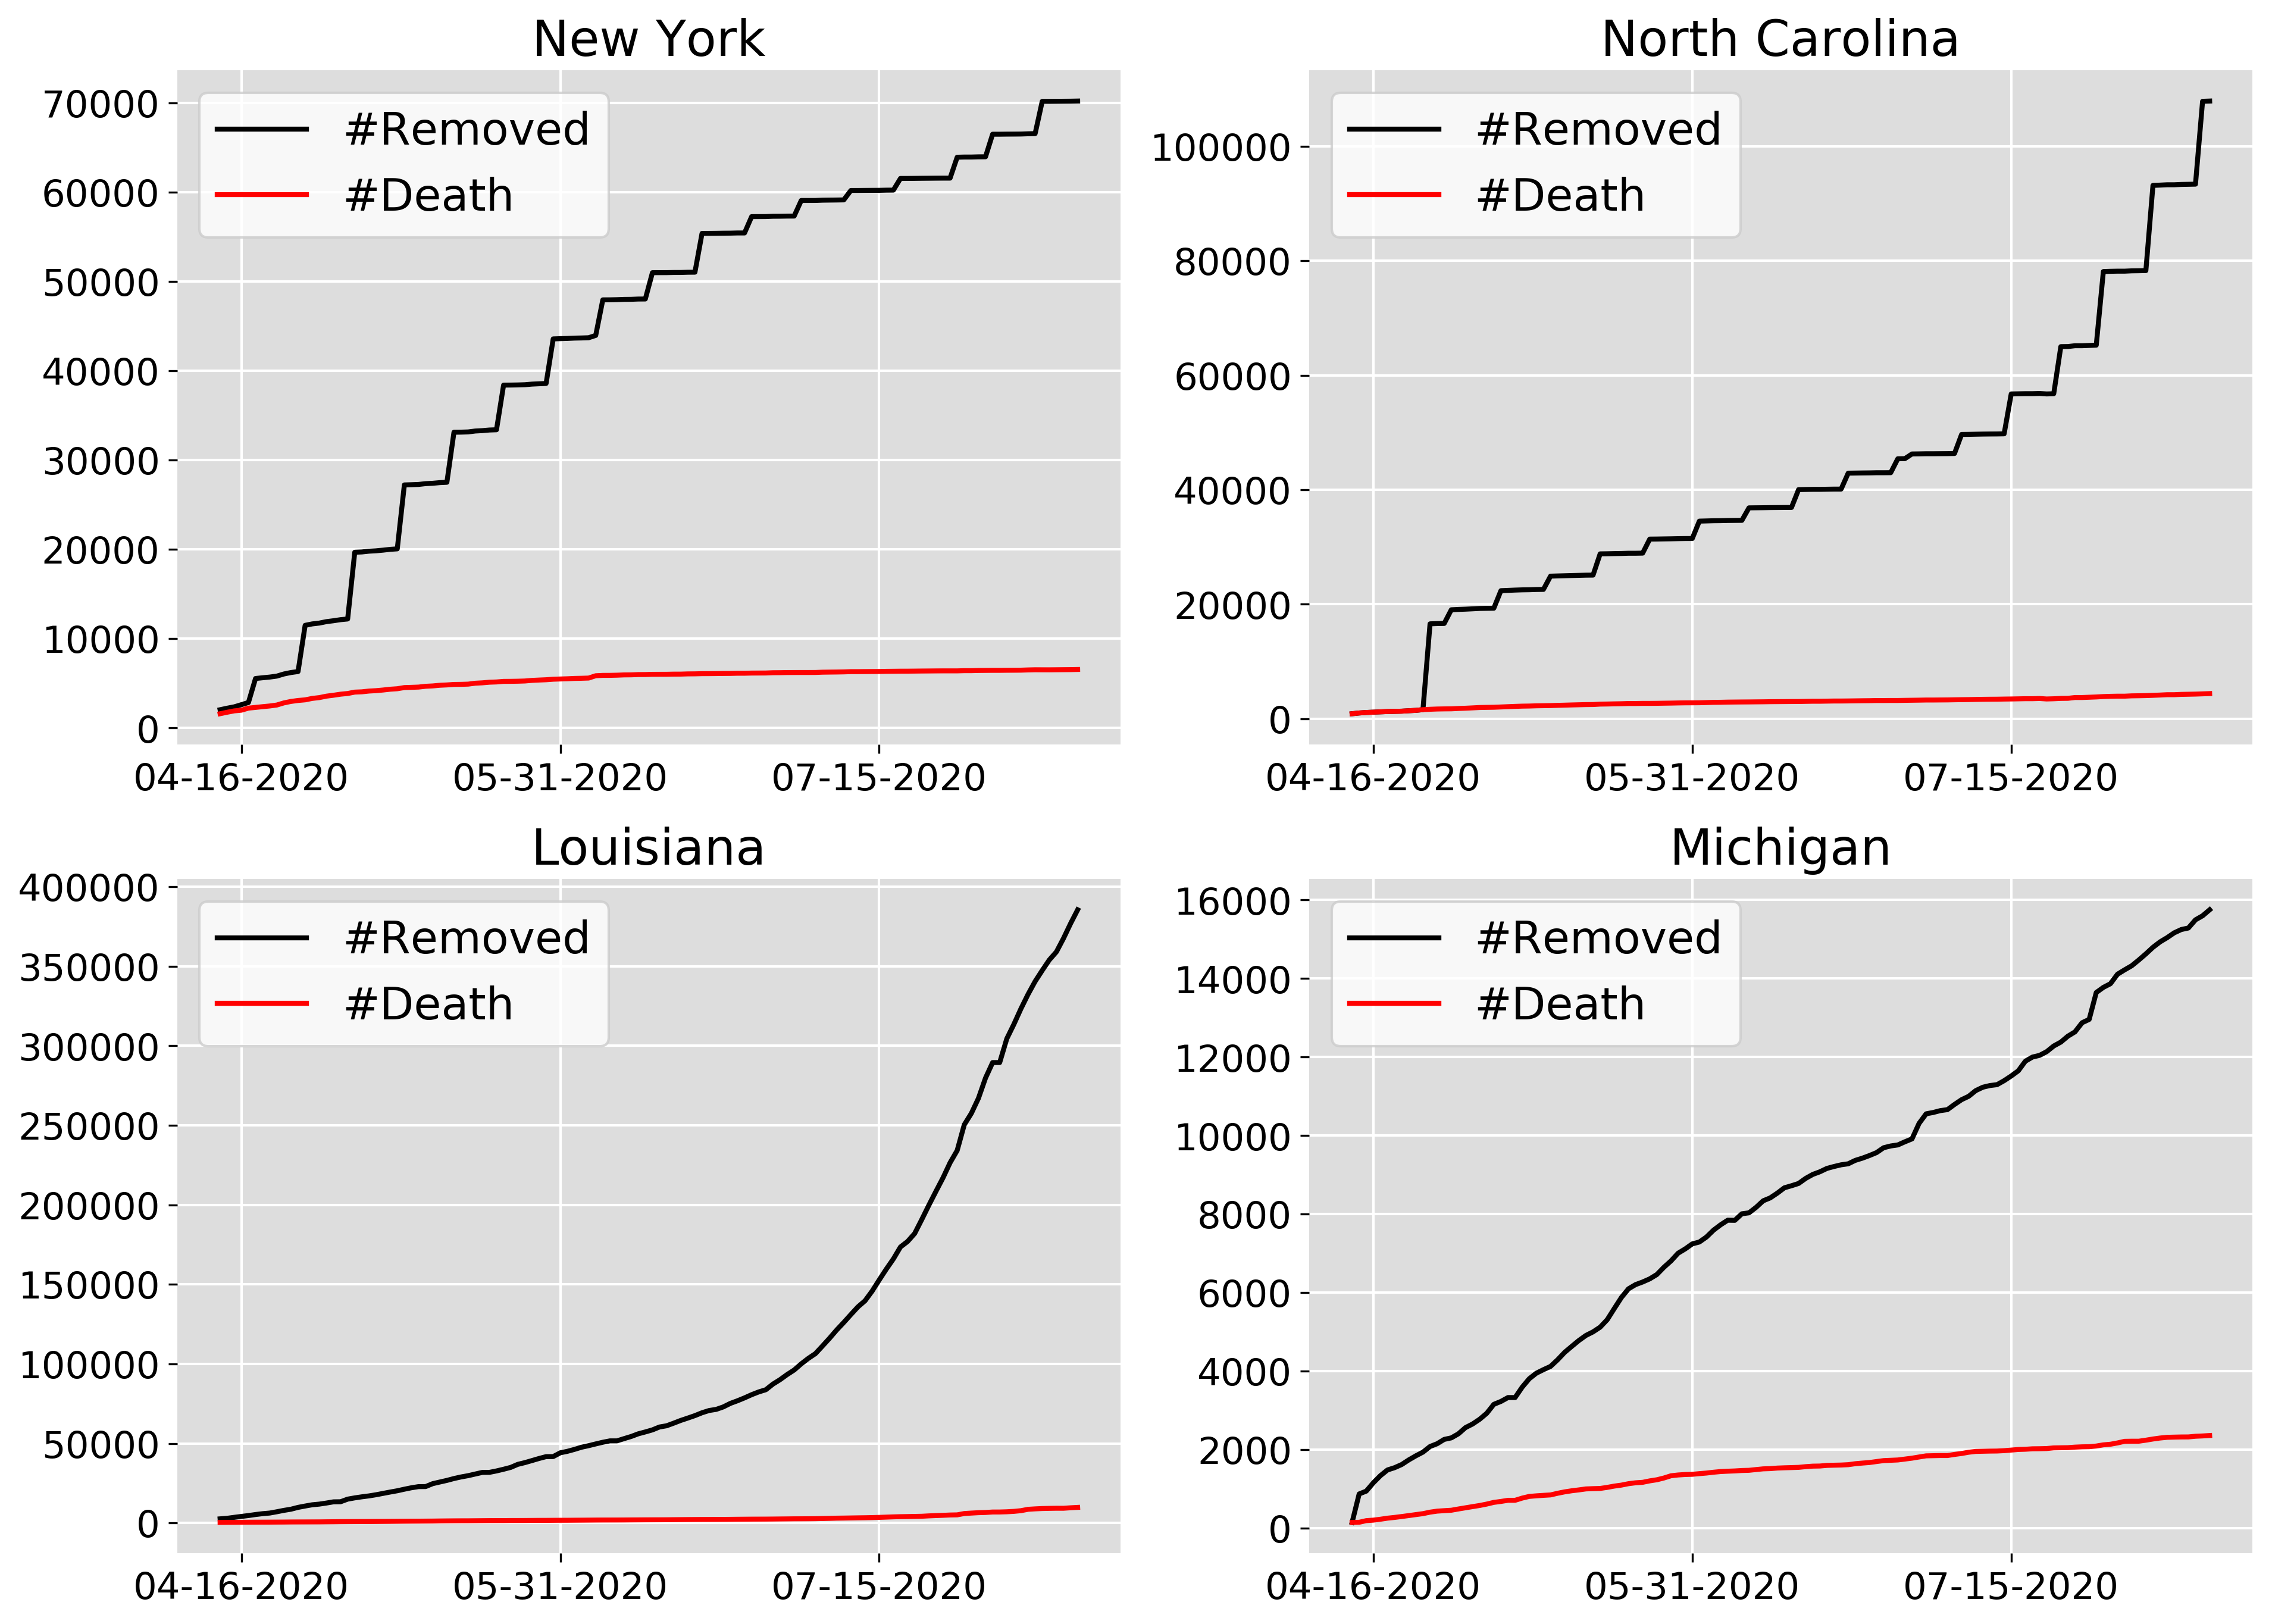}
	\caption{The trajectories of number of accumulated removed and death cases at New York, North Carolina, Louisiana and Michigan.}
	\label{fig:death_rate}
\end{figure}

\begin{figure*}[htb!]
	\centering
	\includegraphics[width=0.32\textwidth]{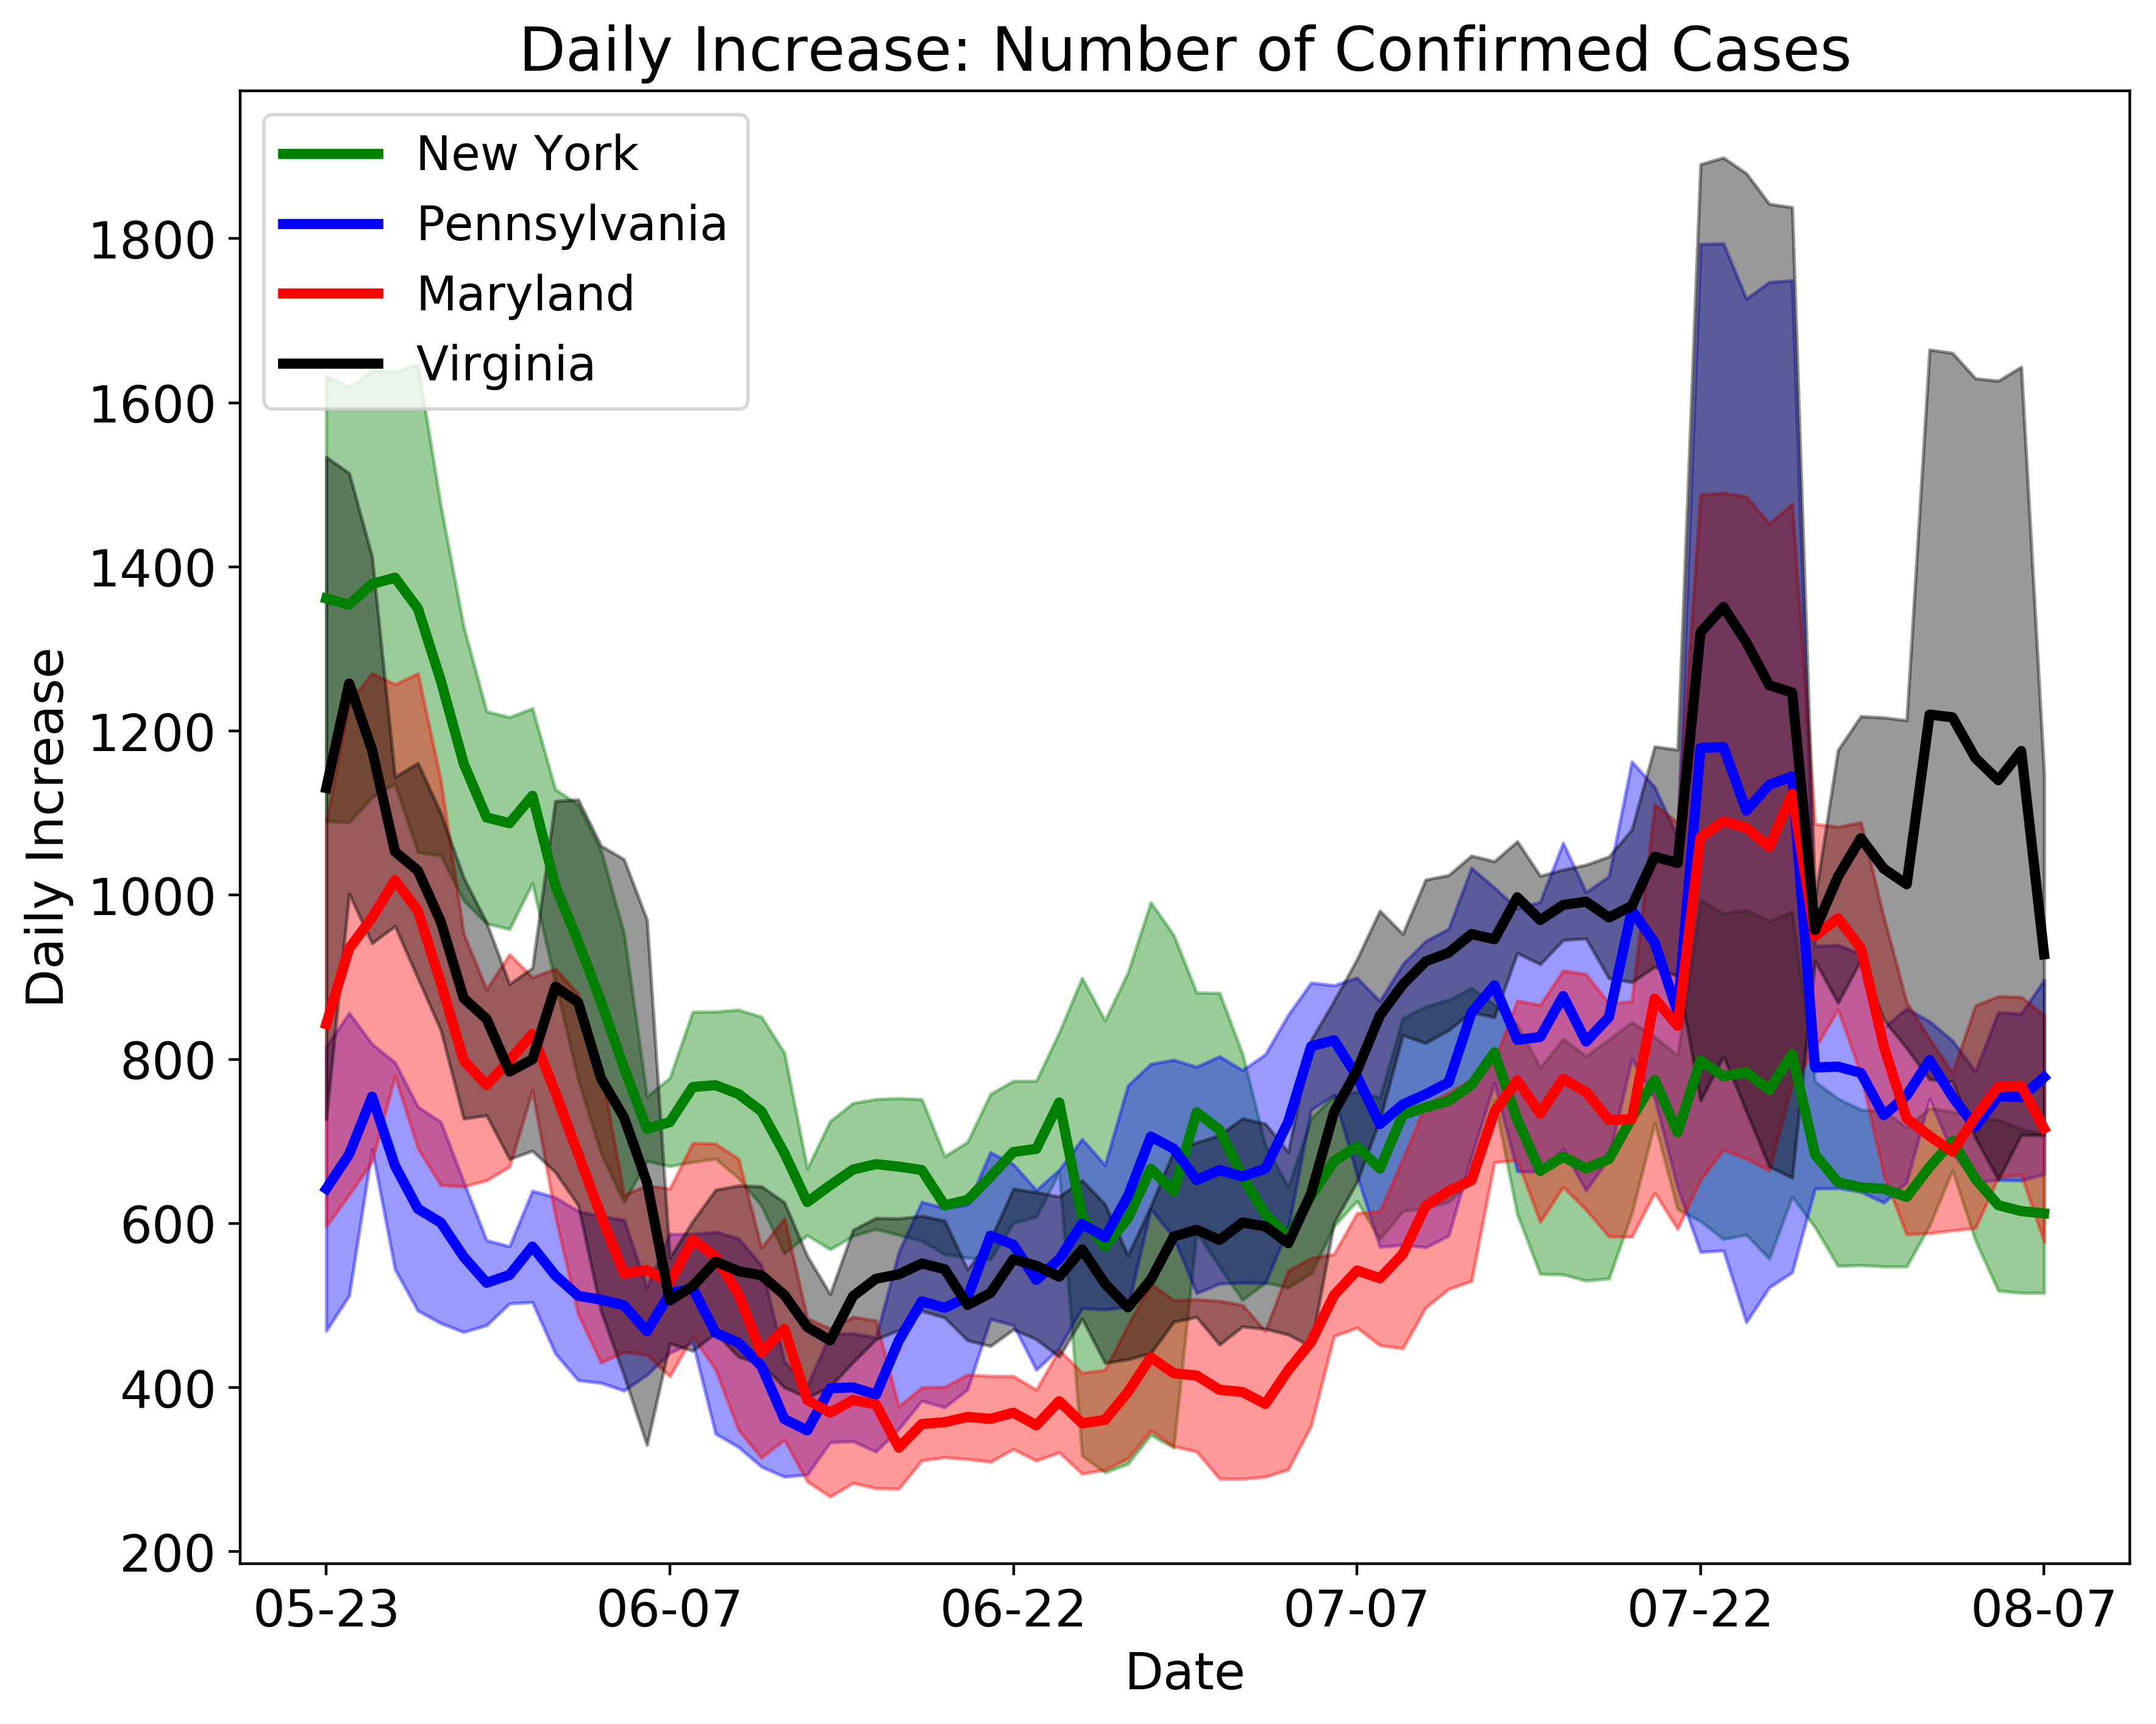}
	\includegraphics[width=0.32\textwidth]{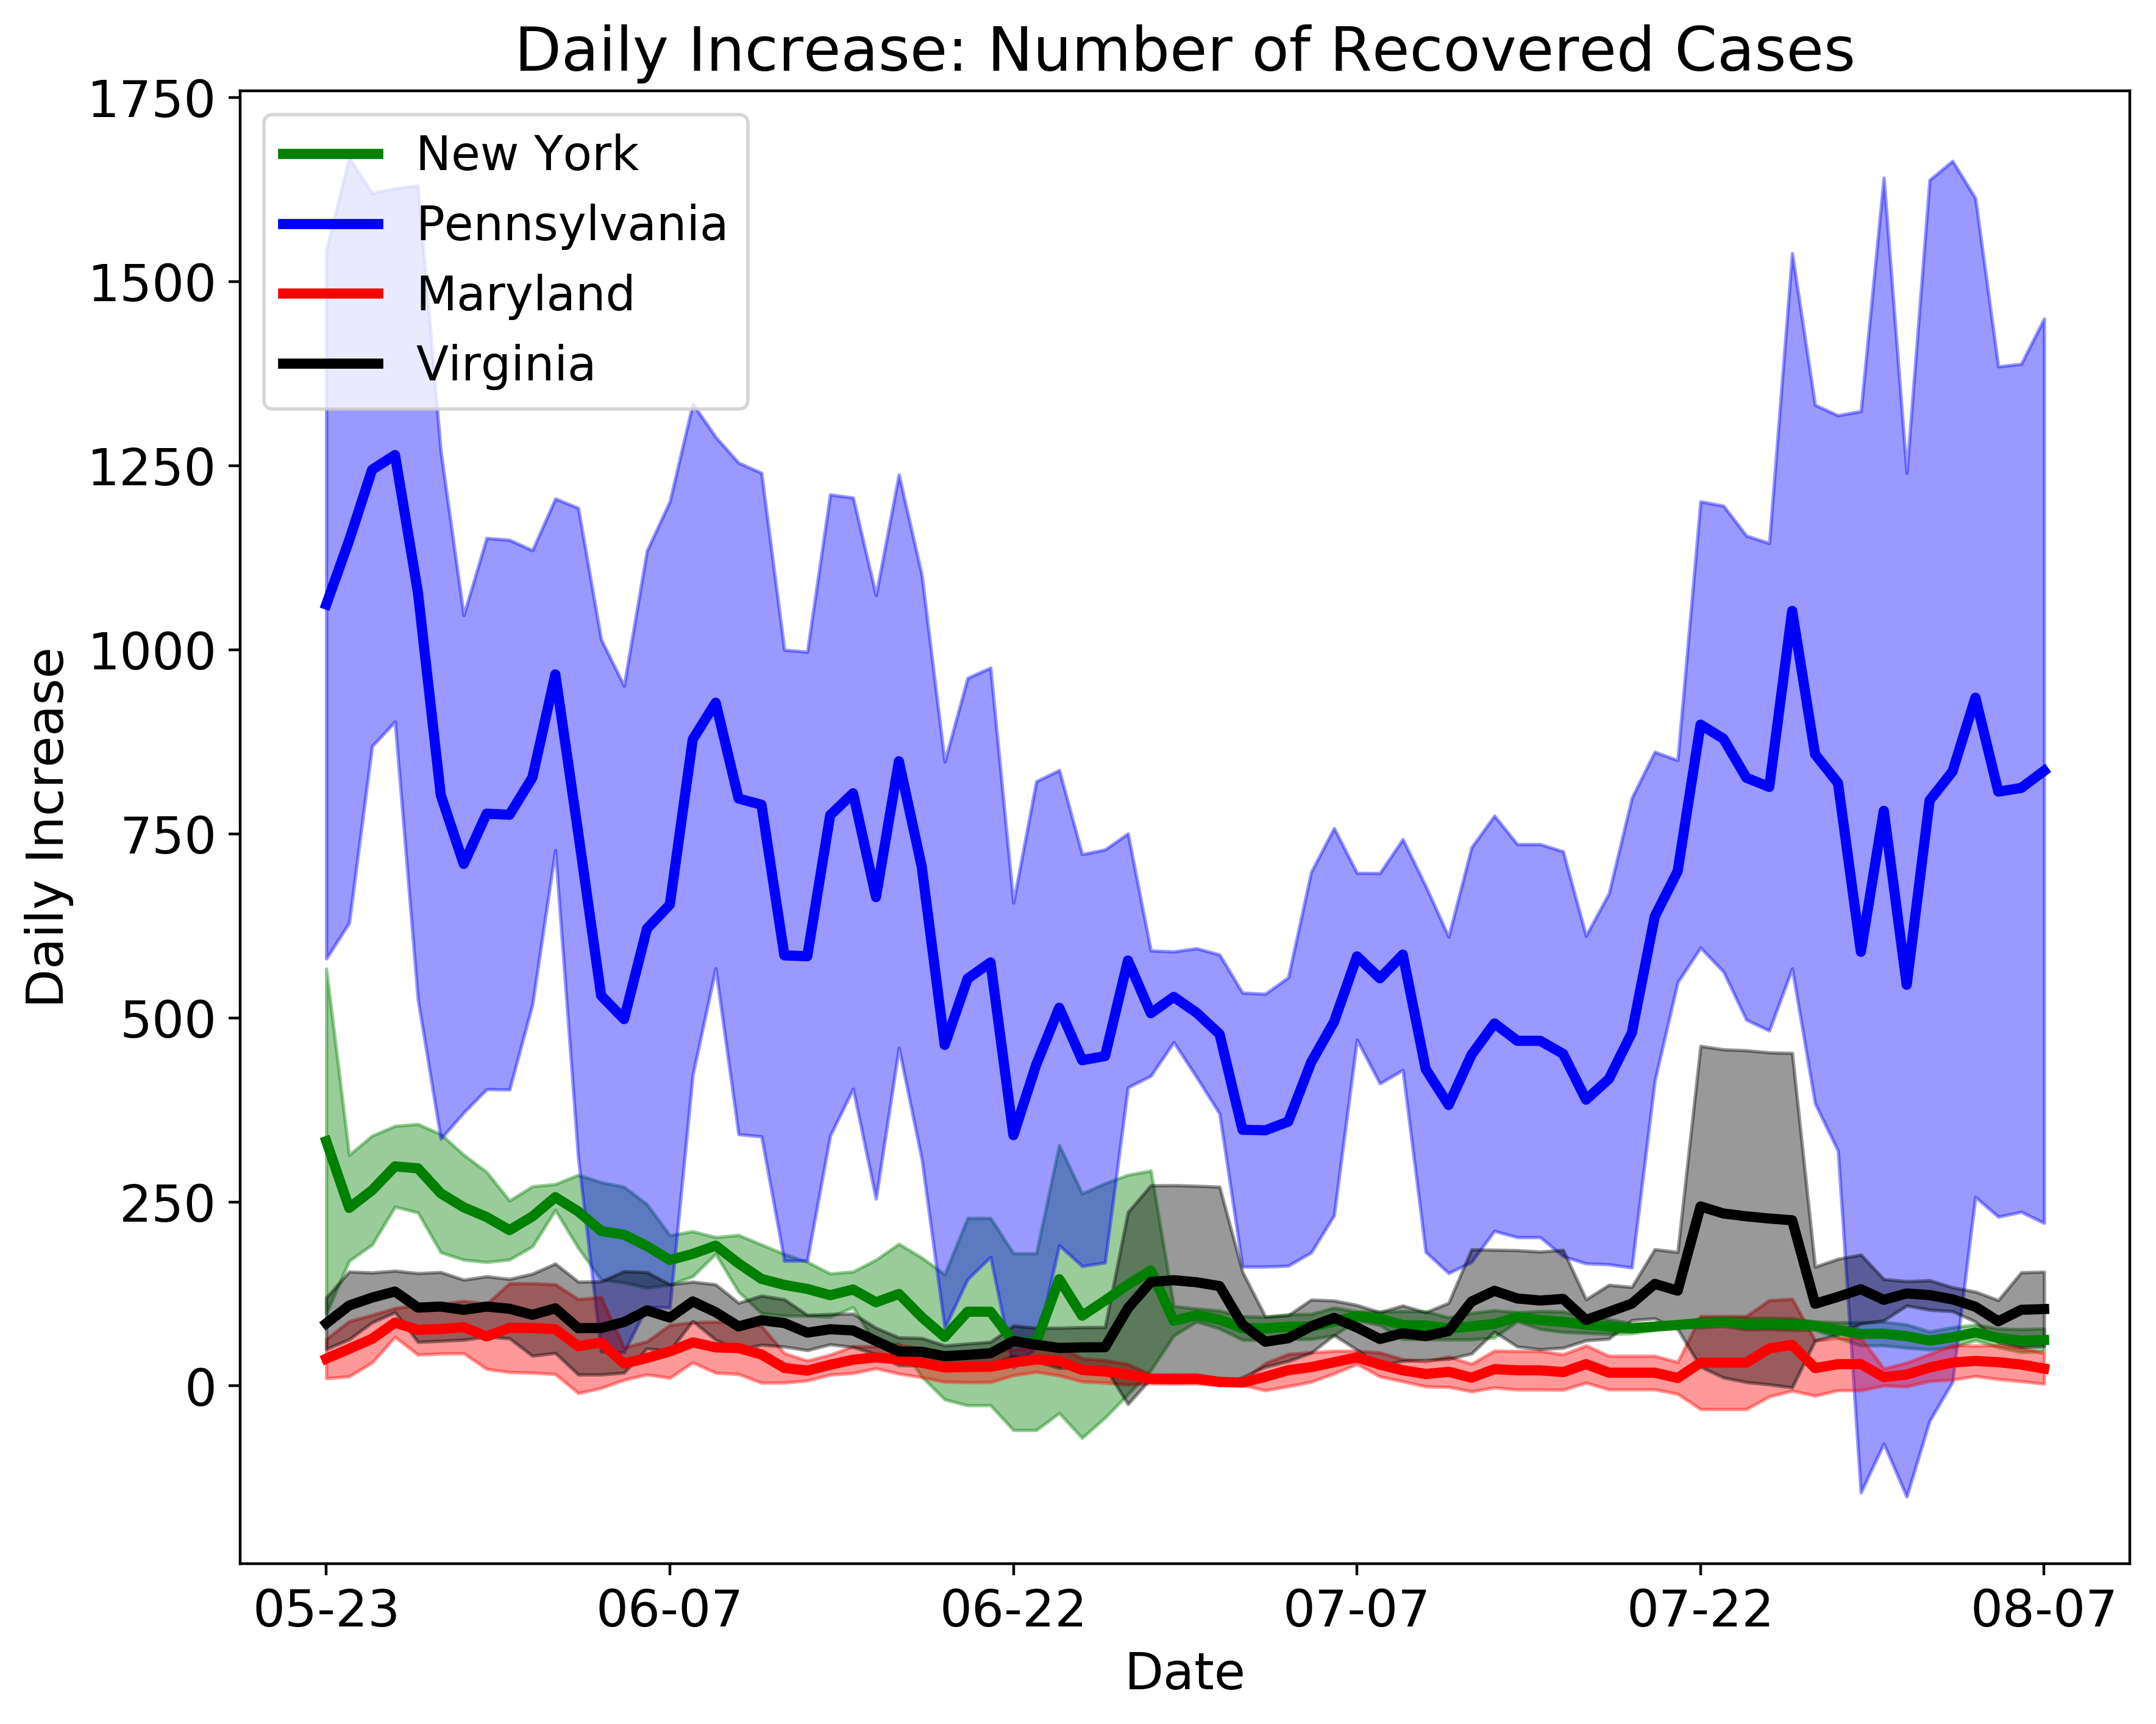}
	\includegraphics[width=0.32\textwidth]{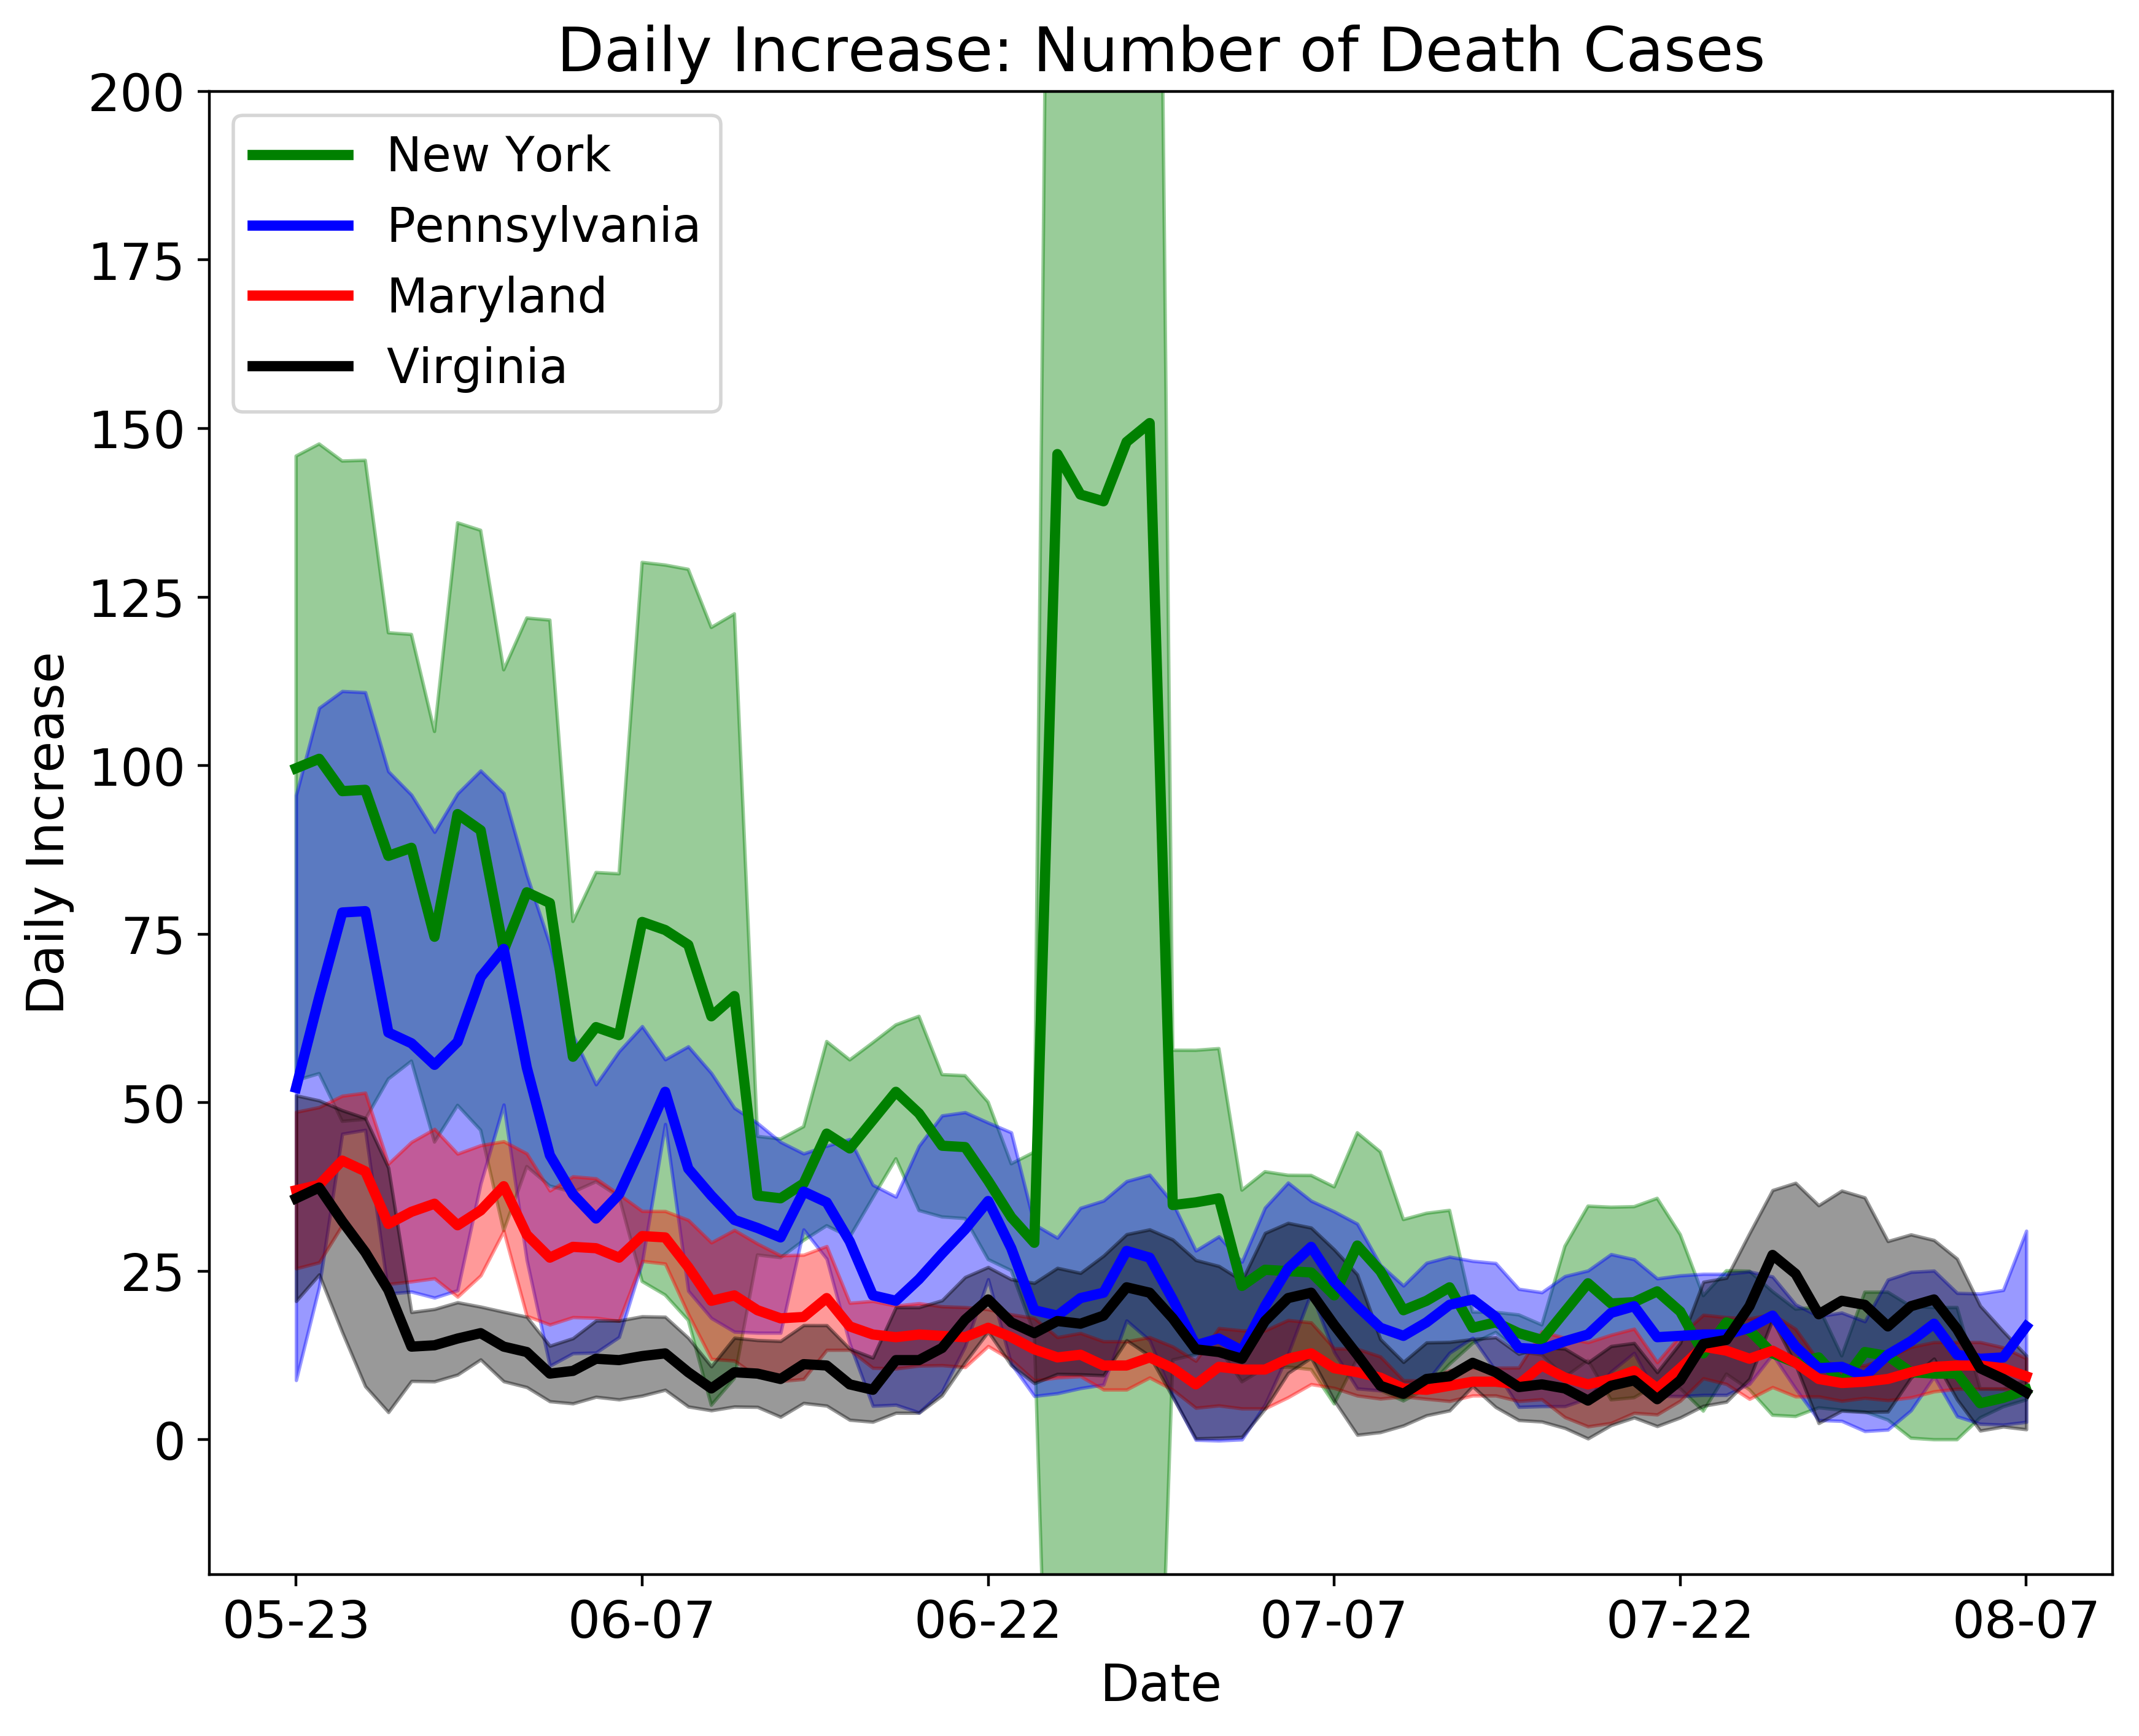}
	\caption{The rolling averages and standard deviation intervals of daily increase time series of four US states. Left: the number of confirmed cases; Middle: the number of recovered cases; Right: the number of death cases}
	\label{covid_data_vis}
\end{figure*}

\section{Numerical Ordinary Differential Equation Solvers}\label{numerical_solver}

Numerical methods are used to solve these coupled ordinary differential equations. Suppose we have an ordinary equation with initial condition,

\begin{equation}
\frac{dy}{dt} = f(t, y),\qquad  y(t_0) = y_0.
\end{equation}

The simplest method to solve this is Euler Method, which a first-order numerical method. It assumes the derivative is constant over a short period to approximate solution.
\begin{equation}
y_{n+1} = y_n + hf(t_n, y_n).
\end{equation}

A more accurate method is Runge-Kutta Method. The following equations shows the 4th order Runge-Kutta Method (RK4). $k_1$ is the slope at the beginning of the interval, if we only use $k1$, then it is just Euler Method. Both $k_2$ and $k_3$ are the slope a the the midpoint of the interval, and $k_4$ is the slope at the end of interval.

\begin{equation}
\begin{dcases}
& y_{n+1} = y_n + \frac{1}{6}f(t_n, y_n),\\
& k_1 = f(t_n, y_n), \\
& k_2 = f(t_n + \frac{h}{2}, y_n + h\frac{k_1}{2}), \\
& k_3 = f(t_n + \frac{h}{2}, y_n + h\frac{k_2}{2}), \\
& k_4 = f(t_n + h, y_n + h k_3).
\end{dcases} 
\end{equation}

\section{Learn synthetic Correlated SuEIR Data}\label{syn_ird}
We generate synthetic 50 correlated time series of length 60 based on Equ \ref{equ_sueird} with the fourth order Runge-Kutta Method. All the parameters in Equ \ref{equ_sueird} are randomly generated. We tried training our model \texttt{AdjMask-SuEIR} given first 10 and 30 steps as input to predict the rest of time series only based on the loss $I$, $R$ and $D$. From Figure \ref{multi_sueir}, we can see that the model is able to correctly learn the trajectories of all six variables given first 30 steps as input. Since there are so many trainable parameters, so we show the mean absolute error between the true parameters and the learned parameters in Table \ref{multi_sueir}. The MAEs of all parameters except for $\bm{\beta}$ and $\bm{A}$ are small because the solutions are not unique. 
\begin{table}[htb!]
\centering
\begin{tabular}{P{1.5cm}|P{2.7cm}|P{2.7cm}}\toprule
\textbf{MAE} & Learned (30) & Learned (10)  \\
\midrule
$\bm{\beta}$  & 0.4635 & 0.3761   \\
\midrule
$\bm{A}$  & 0.3256 & 0.3286   \\
\midrule
$\bm{\gamma}$ & 0.0014 & 0.0003   \\
\midrule
$\bm{\mu}$  & 0.0761 & 0.108  \\
\midrule
$\bm{\sigma}$  & 0.0878 & 0.1213  \\
\midrule
$\bm{E_0}$  & 0.1511 & 0.1782  \\
\midrule
$\bm{S_0}$  & 0.1511 & 0.1873 \\
\bottomrule
\end{tabular}
\caption{The mean absolute error between the true parameters and the learned parameters given 30, 10 steps of training data}
\label{multi_sueir}
\end{table}

\begin{figure}[htb!]
	\centering
	\includegraphics[width=0.4\textwidth]{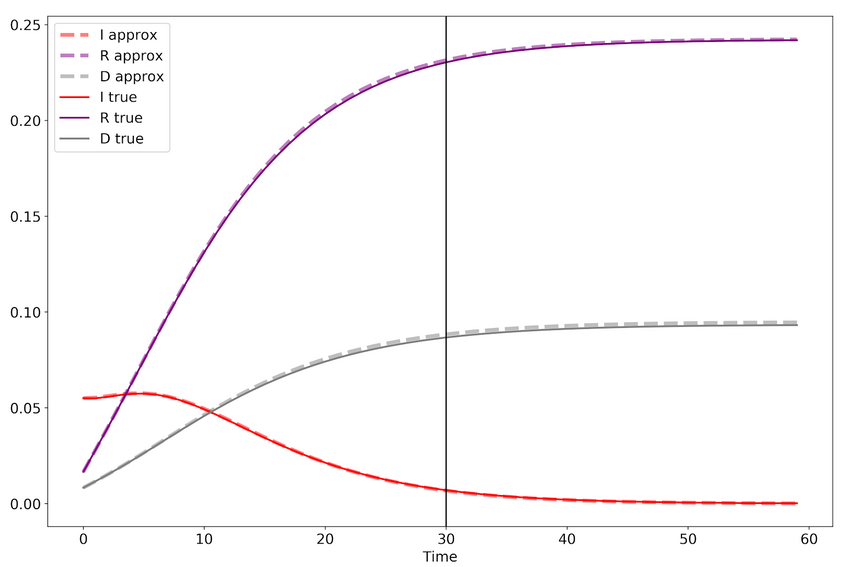}
	\includegraphics[width=0.4\textwidth]{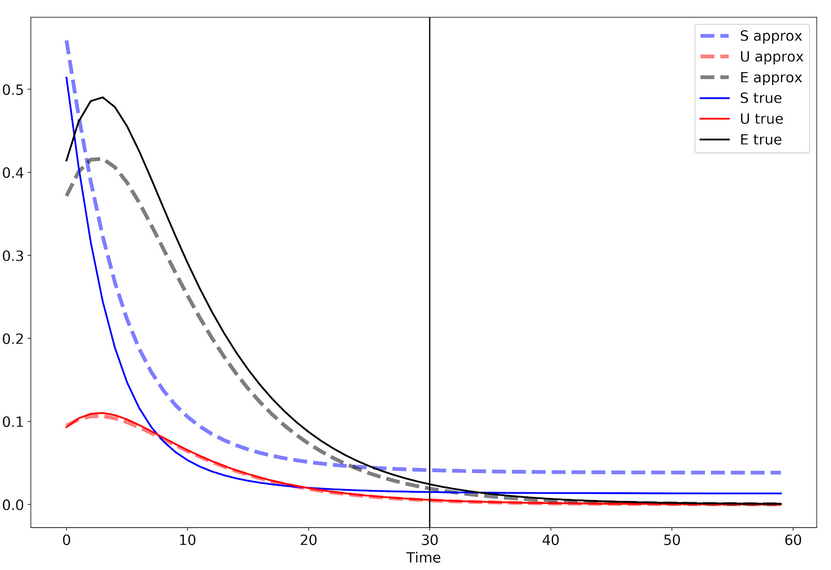}
	\caption{The true and predicted trajectories of five variables in \texttt{Multi-SuEIR} given 30 steps of training data.}
	\label{fig:multi_sueir}
\end{figure}
